# Supplementary material for: Variational Shape Completion for Virtual Planning of Jaw Reconstructive Surgery
Source: arXiv:1906.11957 source file (2019-07-15)
Supplement: Supplementary file 1 [file SupplementaryMaterial.pdf]

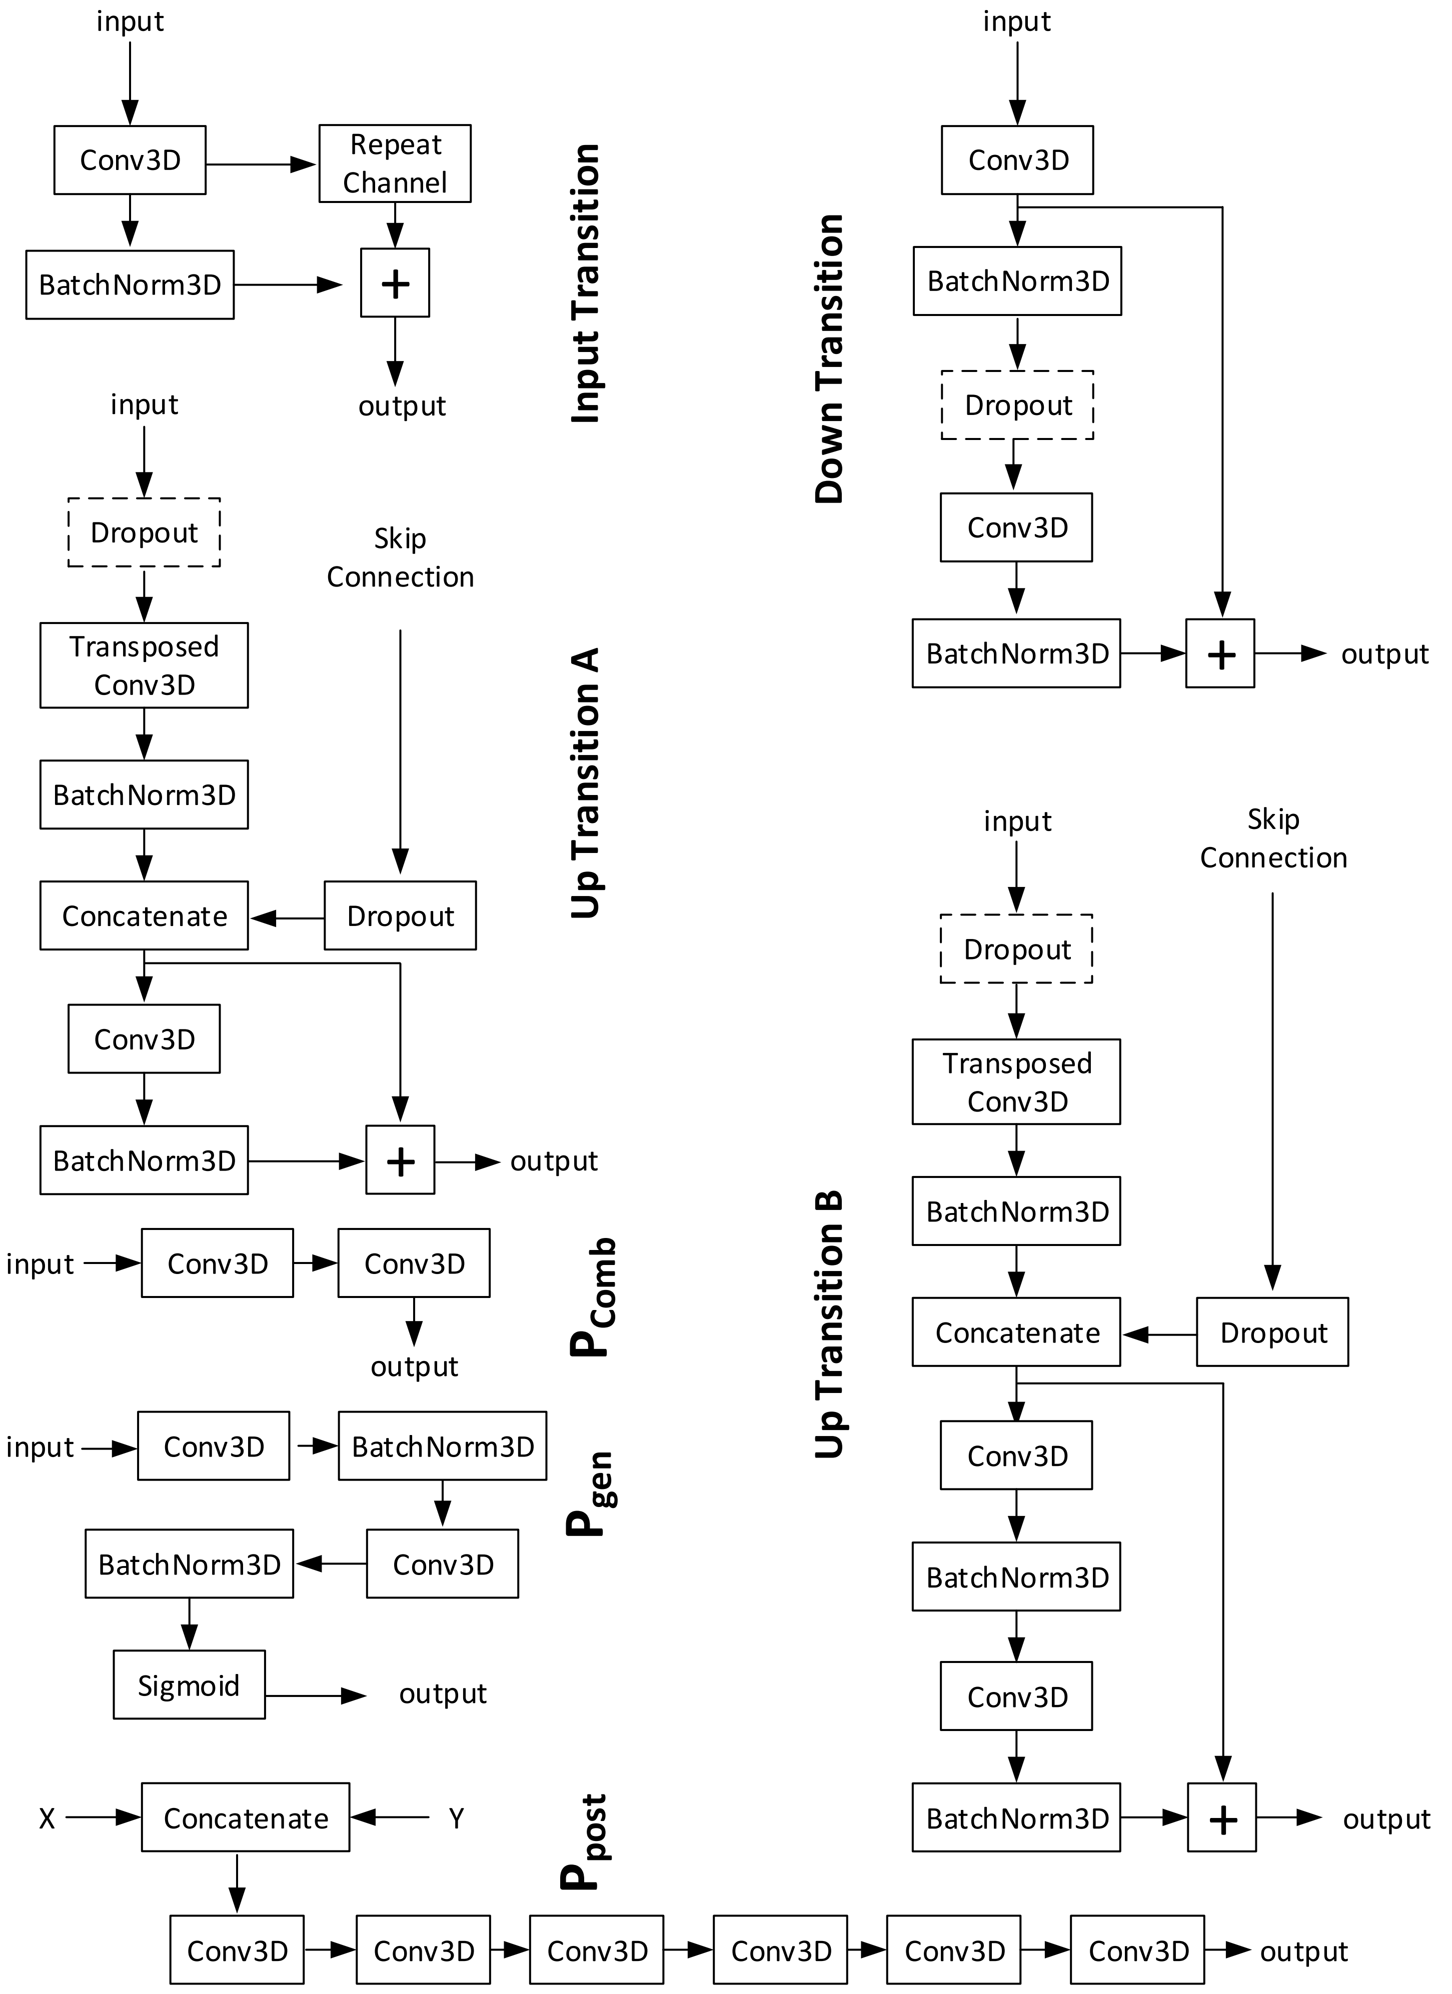


(A)

Supp Figure 1. Details of neural networks. A) Architecture of networks B) Input, output and Intermediate tensors of networks

| Block | Shape of Layer Output |
|---|---|
| Input | $1 \times 141 \times 141 \times 141$ |
| Input Transition | $2 \times 141 \times 141 \times 141$ |
| Down Transition 1 | $4 \times 70 \times 70 \times 70$ |
| Down Transition 2 | $8 \times 35 \times 35 \times 35$ |
| Down Transition 3 | $16 \times 17 \times 17 \times 17$ |
| Down Transition 4 | $32 \times 8 \times 8 \times 8$ |
| Up Transition B1 | $32 \times 17 \times 17 \times 17$ |
| Up Transition B2 | $16 \times 35 \times 35 \times 35$ |
| Up Transition A1 | $8 \times 71 \times 71 \times 71$ |
| Up Transition A2 | $4 \times 141 \times 141 \times 141$ |

Intermediate tensors of the V-Net with its skip connections

| Layer | Shape of Layer Output |
|---|---|
| Input | $12 \times 141 \times 141 \times 141$ |
| Conv1 | $8 \times 141 \times 141 \times 141$ |
| Conv2 | $8 \times 141 \times 141 \times 141$ |

Intermediate tensors of the $P_{Comb}$ Block

| Layer | Shape of Layer Output |
|---|---|
| Input | $4 \mid 8 \times 141 \times 141 \times 141$ |
| Conv1 | $2 \times 142 \times 142 \times 142$ |
| Conv2 | $1 \times 141 \times 141 \times 141$ |

Intermediate tensors of the $P_{gen}$ in the probabilistic (8 input channels) and deterministic (4 input channels) paths

| Layer | Shape of Layer Output |
|---|---|
| Input | $2 \times 141 \times 141 \times 141$ |
| Conv1 | $2 \times 70 \times 70 \times 70$ |
| Conv2 | $4 \times 34 \times 34 \times 34$ |
| Conv3 | $4 \times 16 \times 16 \times 16$ |
| Conv4 | $8 \times 7 \times 7 \times 7$ |
| Conv5 | $8 \times 3 \times 3 \times 3$ |
| Conv6 | $8 \times 1 \times 1 \times 1$ |

Intermediate tensors of the $P_{post}$ Block

(B)

Supp Figure 1 (continued). Details of neural networks. A) Architecture of networks B) Input, output and Intermediate tensors of networks
